# Supplementary material for: Approximate Bayesian Inference via Sparse grid Quadrature Evaluation for Hierarchical Models
Source: arXiv:1904.07270 source file (2019-04-15)
Supplement: Supplementary file 1 [file quadrature_supplement.pdf]

# Supplement to "Approximate Bayesian Inference via Sparse grid Quadrature Evaluation for hierarchical models"

Joshua Hewitt and Jennifer A. Hoeting

Colorado State University

## A Additional posterior quantities

We briefly formulate additional posterior quantities as integrals of functions with respect to the posterior density $f(\boldsymbol{\theta}_2 | \boldsymbol{X})$, which is required for our construction (8).

### A.1 Posterior predictive distributions

Posterior predictive distributions $f(\boldsymbol{X}_0 | \boldsymbol{X})$ naturally fit into the framework described in Section 3.1 because

$$\begin{aligned} f(\boldsymbol{X}_0 | \boldsymbol{X}) &= \int f(\boldsymbol{X}_0, \boldsymbol{\theta}_1, \boldsymbol{\theta}_2 | \boldsymbol{X})\, d(\boldsymbol{\theta}_1, \boldsymbol{\theta}_2) \\ &= \int f(\boldsymbol{X}_0 | \boldsymbol{\theta}_1, \boldsymbol{\theta}_2, \boldsymbol{X})\, f(\boldsymbol{\theta}_1, \boldsymbol{\theta}_2 | \boldsymbol{X})\, d(\boldsymbol{\theta}_1, \boldsymbol{\theta}_2). \end{aligned} \tag{A.1}$$

The posterior predictive distribution (A.1) is exactly a marginal posterior quantity as in (8) for a hierarchical model like (5) in which $\boldsymbol{\theta}_1' = \boldsymbol{X}_0$ and $\boldsymbol{\theta}_2' = (\boldsymbol{\theta}_1, \boldsymbol{\theta}_2)$.

### A.2 Higher order central moments

Posterior variances $\text{Var}(\boldsymbol{\theta}_1 | \boldsymbol{X})$ can be computed with assistance from the law of total variance (9), which uses conditional variances and expectations to facilitate computation. The

decomposition is convenient as conditional variances and expectations may be available in closed form. However, decompositions similar to the law of total variance are not available for general higher order central moments. Approximations must be constructed from the definition of higher order central moments via

$$\mathrm{E}\left[\left(\boldsymbol{\theta}_1 - \mathrm{E}\left[\theta_1 | \boldsymbol{X}\right]\right)^n \middle| \boldsymbol{X}\right] = \int \mathrm{E}_{\boldsymbol{\theta}_1|\boldsymbol{\theta}_2,\boldsymbol{X}}\left[\left(\boldsymbol{\theta}_1 - \mathrm{E}\left[\theta_1 | \boldsymbol{X}\right]\right)^n\right] f\left(\boldsymbol{\theta}_2 | \boldsymbol{X}\right) d\boldsymbol{\theta}_2.$$

The integrand $\mathrm{E}_{\boldsymbol{\theta}_1|\boldsymbol{\theta}_2,\boldsymbol{X}}\left[\left(\boldsymbol{\theta}_1 - \mathrm{E}\left[\theta_1 | \boldsymbol{X}\right]\right)^n\right]$ does not represent a conditional central moment because the moment is centered around the posterior mean $\mathrm{E}\left[\theta_1 | \boldsymbol{X}\right]$ while the expectation is taken with respect to the conditional posterior density $f\left(\boldsymbol{\theta}_1 | \boldsymbol{\theta}_2, \boldsymbol{X}\right)$. If the moment cannot be computed in closed form, approximation strategies may depend on the hierarchical model in question. For example, sparse grid quadrature rules could directly approximate $\mathrm{E}_{\boldsymbol{\theta}_1|\boldsymbol{\theta}_2,\boldsymbol{X}}\left[\left(\boldsymbol{\theta}_1 - \mathrm{E}\left[\theta_1 | \boldsymbol{X}\right]\right)^n\right]$, or it may also be possible to use Laplace approximations.

## A.3 Cumulative distribution functions

Marginal cumulative distribution functions (CDFs) may be formulated as a weighted average of conditional CDFs. The posterior density $f\left(\boldsymbol{\theta}_1 | \boldsymbol{X}\right)$ may be expressed as an integral with respect to $f\left(\boldsymbol{\theta}_2 | \boldsymbol{X}\right)$, and Fubini's theorem allows an exchange of integrals that yield the result via

$$\begin{aligned} F\left(\boldsymbol{\theta}_1 \leq \boldsymbol{t} | \boldsymbol{X}\right) &= \int_{-\infty}^{\boldsymbol{t}} \left( \int f\left(\boldsymbol{\theta}_1 | \boldsymbol{\theta}_2, \boldsymbol{X}\right) f\left(\boldsymbol{\theta}_2 | \boldsymbol{X}\right) d\boldsymbol{\theta}_2 \right) d\boldsymbol{\theta}_1 \\ &= \int F\left(\boldsymbol{\theta}_1 | \boldsymbol{\theta}_2, \boldsymbol{X}\right) f\left(\boldsymbol{\theta}_2 | \boldsymbol{X}\right) d\boldsymbol{\theta}_2. \end{aligned}$$

## A.4 Information criteria

The Deviance information criteria (DIC, Spiegelhalter, Best, Carlin, & van der Linde, 2002) allows for model comparison and is based on the deviance, defined via

$$D(\boldsymbol{\theta}_1, \boldsymbol{\theta}_2) = -2 \ln f(\boldsymbol{X} \mid \boldsymbol{\theta}_1, \boldsymbol{\theta}_2) + C$$

for a constant $C$ that depends on the data. The DIC is defined via

$$\mathrm{DIC} = \mathrm{E}\left[D(\boldsymbol{\theta}_1, \boldsymbol{\theta}_2) \mid \boldsymbol{X}\right] + p_D,$$

in which $p_D = \mathrm{E}\left[D(\boldsymbol{\theta}_1, \boldsymbol{\theta}_2) \mid \boldsymbol{X}\right] - D\left(\mathrm{E}\left[\boldsymbol{\theta}_1 \mid \boldsymbol{X}\right], \mathrm{E}\left[\boldsymbol{\theta}_2 \mid \boldsymbol{X}\right]\right)$. Only the posterior expectation $\mathrm{E}\left[D(\boldsymbol{\theta}_1, \boldsymbol{\theta}_2) \mid \boldsymbol{X}\right]$ requires additional formulation. The law of total expectation yields an integral with respect to $f(\boldsymbol{\theta}_2 \mid \boldsymbol{X})$ via

$$\mathrm{E}\left[D(\boldsymbol{\theta}_1, \boldsymbol{\theta}_2) \mid \boldsymbol{X}\right] = \int \mathrm{E}_{\boldsymbol{\theta}_1 \mid \boldsymbol{\theta}_2, \boldsymbol{X}}\left[D(\boldsymbol{\theta}_1, \boldsymbol{\theta}_2)\right] f(\boldsymbol{\theta}_2 \mid \boldsymbol{X})\, d\boldsymbol{\theta}_2.$$

Similar to the formulation of higher order central moments (Section A.2), closed form expressions may be available for the integrand $\mathrm{E}_{\boldsymbol{\theta}_1 \mid \boldsymbol{\theta}_2, \boldsymbol{X}}\left[D(\boldsymbol{\theta}_1, \boldsymbol{\theta}_2)\right]$, or it may need to be approximated directly via sparse grid quadrature rules or via Laplace approximations. The Watanabe-Akaike information criterion (WAIC) uses similar quantities as the DIC, so may be similarly approximated (Watanabe, 2010).

# B Additional computational techniques

BISQuE approximations use weighted sums of densities and likelihoods, however, it is often more numerically stable to evaluate log-densities and log-likelihoods. This section reviews techniques that allow log-densities and log-likelihoods to be used to compute weighted sums of densities.

## B.1 Evaluating an unnormalized density

Let $f(x)$ be a probability density function such that $f(x) \propto g(x)$ for some unnormalized density function $g(x)$. If $g(x)$ or $\ln g(x)$ are known, then one strategy to evaluate $f(x)$ is to first compute the integration constant $C = \int g(x)\, dx$. In special cases, quadrature techniques can efficiently approximate the integration constant $C$. However, the numerical stability of such approximations are often better when $\ln g(x)$ is used to compute $kC$ for some scale factor $k > 0$. An $m$ point quadrature rule with quadrature nodes $\left\{x^{(i)} : i = 1, \ldots, m\right\}$ and weights $\{w_i : i = 1, \ldots, m\}$ approximates the scaled constant $kC$ via

$$kC = \int \exp\{\ln g(x) + \ln k\}\, dx \approx \sum_{i=1}^{m} \exp\left\{\ln g\left(x^{(i)}\right) + \ln k\right\} w_i. \tag{B.1}$$

Choosing $k$ can be difficult, but the approximation (B.1) suggests that $k$ such that $\ln k = -m^{-1} \sum_{i=1}^{m} \ln g\left(x^{(i)}\right)$ will often be a reasonable choice since $\ln k$ centers the shifted unnormalized log-densities $\left\{\ln g\left(x^{(i)}\right) + \ln k : i = 1, \ldots, m\right\}$ around 0. The integration constant $C$ can be recovered via $C = \exp\{\ln kC - \ln k\}$ after $kC$ and $\ln k$ are numerically evaluated.

## B.2 Evaluating mixture densities

Let $f(x)$ be a mixture of densities $\{f_i(x) : i = 1, \ldots, m\}$ with weights $\{w_i : i =, \ldots, m\}$ specified via

$$f(x) = \sum_{i=1}^{m} f_i(x)\, w_i.$$

One strategy for evaluating $f(x)$ is to again introduce a scale factor $k > 0$. This allows for numerically stable evaluation of $f(x)$ via

$$f(x) = \frac{kf(x)}{k} = \frac{\sum_{i=1}^{m} \exp\{\ln f_i(x) + \ln k\}\, w_i}{k}.$$

Choosing $k$ can be difficult, but as in Section B.1, $k$ such that $\ln k = -m \sum_{i=1}^{m} \ln f_i(x)$ will often be reasonable.

# C Derivations for examples

## C.1 Fur seals

We derive components required for the BISQuE approximations of posterior quantities for the fur seals example, as specified in Table 2.

### C.1.1 Joint posterior

The joint posterior density is known up to a proportionality constant via

$$
\begin{aligned}
f(N, \boldsymbol{\alpha}, \theta_1, \theta_2 | \boldsymbol{c}, r) &\propto f(\boldsymbol{c}, r | N, \boldsymbol{\alpha}) f(N) f(\boldsymbol{\alpha} | \theta_1, \theta_2) f(\theta_1, \theta_2) \\
&\propto \frac{(N-1)!}{(N-r)!} \frac{\exp\{-(\theta_1+\theta_2)/1000\}}{B(\theta_1, \theta_2)^I} \prod_{i=1}^{I} \alpha_i^{c_i+\theta_1-1} (1-\alpha_i)^{N-c_i+\theta_2-1},
\end{aligned}
\tag{C.1}
$$

in which $B(\theta_1, \theta_2) = \Gamma(\theta_1)\Gamma(\theta_2)/\Gamma(\theta_1+\theta_2)$ is the beta function.

### C.1.2 Population size

The BISQuE approximation for $f(N|\boldsymbol{c}, r)$ uses the two conditional posterior densities $f(N-r|\boldsymbol{\alpha}, \theta_1, \theta_2, \boldsymbol{c}, r)$ and $f(\boldsymbol{\alpha}, \theta_1, \theta_2 | \boldsymbol{c}, r)$, which are derived from the joint posterior density (C.1). Factoring (C.1) yields

$$
f(N|\boldsymbol{\alpha}, \theta_1, \theta_2, \boldsymbol{c}, r) \propto \frac{(N-1)!}{(N-r)!} \prod_{i=1}^{I} (1-\alpha_i)^N,
$$

which implies the change of variable $k = N - r$ yields the result

$$
f(N-r|\boldsymbol{\alpha}, \theta_1, \theta_2, \boldsymbol{c}, r) \sim \text{Neg. Bin.}\left(r, 1 - \prod_{i=1}^{I}(1-\alpha_i)\right).
$$

The posterior density $f(\boldsymbol{\alpha}, \theta_1, \theta_2 | \boldsymbol{c}, r)$ may be computed by marginalizing (C.1) with respect to $N$, via

$$\text{(C.2)} \quad f(\boldsymbol{\alpha}, \theta_1, \theta_2 | \boldsymbol{c}, r) \propto \sum_{N=r}^{\infty} f(N, \boldsymbol{\alpha}, \theta_1, \theta_2 | \boldsymbol{c}, r)$$
$$\propto h(\boldsymbol{\alpha}) \frac{\exp\{-(\theta_1 + \theta_2)/1000\}}{B(\theta_1, \theta_2)^I} \prod_{i=1}^{I} \alpha_i^{c_i + \theta_1 - 1} (1 - \alpha_i)^{\theta_2 - c_i - 1},$$

in which

$$h(\boldsymbol{\alpha}) = \sum_{N=r}^{\infty} \frac{(N-1)!}{(N-r)!} (1-p)^N$$
$$\propto (1-p)^r p^{-r} \sum_{k=0}^{\infty} \binom{k+r-1}{r-1} (1-p)^k p^r$$
$$\propto (1-p)^r p^{-r}$$

for $1 - p = \prod_{i=1}^{I} (1 - \alpha_i)$ and the change of variable $k = N - r$. The marginalized posterior may be simplified further since (C.2) contains kernels for Beta distributions. Thus,

$$\text{(C.3)} \quad f(\boldsymbol{\alpha}, \theta_1, \theta_2 | \boldsymbol{c}, r) \propto \frac{\exp\{-(\theta_1 + \theta_2)/1000\}}{B(\theta_1, \theta_2)^I} \times$$
$$p^{-r} \prod_{i=1}^{I} B(\theta_1 + c_i, \theta_2 + r - c_i) f(\alpha_i | \theta_1 + c_i, \theta_2 + r - c_i).$$

### C.1.3 Capture probabilities

The BISQuE approximation for $f(\alpha_i | \boldsymbol{c}, r)$ uses the posterior densities $f(\alpha_i | N, \theta_1, \theta_2)$ and $f(N, \theta_1, \theta_2 | \boldsymbol{c}, r)$. Factoring (C.1) immediately yields

$$f(\alpha_i | N, \theta_1, \theta_2) \sim \text{Beta}(\theta_1 + c_i, \theta_2 + N - c_i).$$

Similarly, marginalizing (C.1) with respect to $\boldsymbol{\alpha}$ immediately yields

$$f\left(N, \theta_1, \theta_2 \middle| \boldsymbol{c}, r\right) \propto \frac{(N-1)!}{(N-r)!} \frac{\exp\left\{-\left(\theta_1+\theta_2\right)/1000\right\}}{B\left(\theta_1, \theta_2\right)^I} \prod_{i=1}^{I} B\left(\theta_1 + c_i, \theta_2 + N - c_i\right).$$

### C.1.4 Hyperparameters

The BISQuE approximation for $f\left(U_1 \middle| \boldsymbol{c}, r\right)$ uses the posterior densities $f\left(\theta_1, \theta_2 \middle| \boldsymbol{\alpha}, \boldsymbol{c}, r\right)$ and $f\left(\boldsymbol{\alpha} \middle| \boldsymbol{c}, r\right)$. Factoring (C.3) yields

$$f\left(\theta_1, \theta_2 \middle| \boldsymbol{\alpha}, \boldsymbol{c}, r\right) \propto \frac{\exp\left\{-\left(\theta_1+\theta_2\right)/1000\right\}}{B\left(\theta_1, \theta_2\right)^I} \prod_{i=1}^{I} \alpha_i^{\theta_1} \left(1-\alpha_i\right)^{\theta_2}.$$

The marginal posterior $f\left(\boldsymbol{\alpha} \middle| \boldsymbol{c}, r\right)$ must be approximated via nested integration, and is specified via

$$f\left(\boldsymbol{\alpha} \middle| \boldsymbol{c}, r\right) \propto p^{-r} \left(\prod_{i=1}^{I} \alpha_i^{c_i-1} \left(1-\alpha_i\right)^{r-c_i-1}\right) \int f\left(\theta_1, \theta_2 \middle| \boldsymbol{\alpha}, \boldsymbol{c}, r\right) d\left(\theta_1, \theta_2\right).$$

# References

Spiegelhalter, D. J., Best, N. G., Carlin, B. P., & van der Linde, A. (2002). Bayesian measures of model complexity and fit. *Journal of the Royal Statistical Society Series B*, *64*(4), 583–639.

Watanabe, S. (2010). Asymptotic Equivalence of Bayes Cross Validation and Widely Applicable Information Criterion in Singular Learning Theory. *Journal of Machine Learning Research*, *11*, 3571–3594.
